# Supplementary material for: Investigating the Effects of Mood & Usage Behaviour on Notification Response Time
Source: arXiv:2207.03405 source file (2022-07-07)
Supplement: Supplementary file 1 [file appendix.tex]

%----------------------------------------------------------------------------------
%	Appendix
%----------------------------------------------------------------------------------
\section{Appendix}
